# Supplementary material for: Tree tensor network hierarchical equations of motion based on time-dependent variational principle for efficient open quantum dynamics in structured thermal environments
Source: arXiv:2505.00126 source file (2025-07-30)
Supplement: Supplementary file 1 [file si.pdf]

# Supplementary Material: Tree tensor network hierarchical equations of motion based on time-dependent variational principle for efficient open quantum dynamics in structured thermal environments

Xinxian Chen*

*Department of Chemistry, University of Rochester, Rochester, New York 14627, USA*

Ignacio Franco†

*Department of Chemistry, University of Rochester,*
*Rochester, New York 14627, United States and*
*Department of Physics, University of Rochester,*
*Rochester, New York 14627, United States*

(Dated: April 30, 2025)

In this Supplementary Material, we offer the theory and algorithm of the tree tensor network (TTN) decomposition of a general master equation with a summation-of-product form, including the hierarchical equations of motion. The TTN admits a general tree topology described with the help of graph notations.

For simplicity, we assume Einstein's summation convention throughout this Supplementary Material.

## I. NOTATIONS

In a TTN decomposition, a $K$-order tensor $\Omega$ is decomposed by contracting several lower-order *core tensors*. Generally, for high-order tensors, such a decomposition is not unique. For clarity, we call the index $i_1, \ldots, i_K$ in the high-order tensor $\Omega_{i_1 \cdots i_K}$ as the *primitive index*, while the indexes in core tensors that are not primitive are *contracted*. To discuss different tensor network methods and the corresponding propagation schemes, it is convenient to use a tree graph $G$ to represent the topology of a tensor network. In this representation, each node in $G$ corresponds to a core tensor in the decomposition, each closed edge in $G$ corresponds to an index to be contracted, and each open edge to be a primitive index.

We define a *graph* $G = (V, E, R)$ as a tuple of a finite *node* set $V$, an *edge* set $E$, and a *relation* map $R\colon V \mapsto 2^E$ that describes the connectivity in the graph, where $2^E = \{U \mid U \subseteq E\}$ is the power set of $E$. The number of edges in $R(v)$ is the *degree* of $v$. The edges are assumed to be unidirectional, and connected to either one node or two different vertices. For any two vertices there is at most one edge between them. That is, for any edge in $e \in E$, we can only find either one or two different vertices $v_i$ such that $e \in R(v_i)$, and we call such an edge $e$ to be *open* for the former case and call it *closed* for the latter one. For a closed edge $e$, if $u \neq v$ such that $e \in R(u)$ and $e \in R(v)$ then we say $u$ and $v$ is *contracted* by $e$. The *neighborhood* of a node $\mathcal{N}(v)$ is defined as $\{v_i \in V,\ v_i \neq v \mid \exists e \in R(v) \text{ s.t. } e \in R(v_i)\}$. A *path* from node $a$ to $b$ is a non-empty sequence of different vertices $(x_0, \ldots, x_L)$ that satisfies $x_0 = a$, $x_N = b$ and $x_\ell \in \mathcal{N}(x_{\ell-1})$ for $\ell = 1, \ldots, L$, with $L$ the *length* of the sequence. The graph is assumed to be connected in this paper. That is, for any two different vertices in $V$ we can find a path that connects them. A graph is called a *tree* if such a path is unique for any two different vertices. The concept of tree-like hierarchy can be constructed once

* xchen106@ur.rochester.edu

† ignacio.franco@rochester.edu

one node $r$ in the tree is defined as the *root* of the tree. Since the tree is connected, for any $u \in V$ and $u \neq r$ we can find a path from $r$ to $u$ with length denoted as $\mathsf{L}_{G,r}(u)$. Here $\mathsf{L}_{G,r}(u)$ is named as the *height* of node $u$ in the tree $G$ with root $r$. Specially, $\mathsf{L}_{G,r}(r) = 0$. Once the root $r$ is determined, for a node $u \neq r$, we call the edge $a \in R(u)$ as the *parent edge* of $u$ if $a \in R(v)$ and $\mathsf{L}_{G,r}(v) = \mathsf{L}_{G,r}(u) - 1$, and $v$ is the *parent* of $u$.

## II. HIERARCHICAL TUCKER DECOMPOSITION FOR A HIGH ORDER TENSOR

The decomposition of a high-order tensor can be considered from the hierarchical partition of its indexes. A *partition* of a set is a grouping of some elements into non-empty subsets, in such a way that every grouped element is included in exactly one subset. A *hierarchical partition* is to repeat the process above for the generated subset finite multiple times. For example, $\{\{i,\ j\},\ \{k,\ l\}\}$ is a partition of $\{i,\ j,\ k,\ l\}$ and $\{i,\ \{j,\ \{k,\ \{l\}\}\}\}$ is a hierarchical one. Obviously, the (hierarchical) partition of a set is usually not unique.

For a $K$-order tensor $\Omega_{i_1\cdots i_K}$ with $i_k = 1,\ \ldots,\ N_k$ for $k = 1,\ \ldots,\ K$, $N_k$ is the *dimension* of the primitive index $i_k$. This high-tensor can be rearranged into a matrix manifold as $\Omega_{I^{(1)}J^{(1)}}$, with $\left\{I^{(1)},\ J^{(1)}\right\}$ a partition of the set of primitive indexes $i_1,\ \ldots,\ i_K$. From the SVD the matrix $\Omega_{IJ}$ can be decomposed into $\Omega_{I^{(1)}J^{(1)}} = U_{I^{(1)}a_1}\Lambda_{a_1}V^\star_{Ja_1} = U_{I^{(1)}a_1}C^{(1)}_{a_1J^{(1)}}$. Note that we can perform the same procedure iteratively. From the SVD the matrix manifold $\Omega_{IJ}$ can be decomposed into $\Omega_{I^{(1)}J^{(1)}} = U_{I^{(1)}a_1}\Lambda_{a_1}V^\star_{Ja_1} = U_{I^{(1)}a_1}C^{(1)}_{a_1J^{(1)}}$. That is, from $C^{(1)}_{a_1J^{(1)}}$ for a given $a_1$ we get $C^{(2)}_{a_1a_2J^{(2)}}$, and $U_{I^{(2)}a_2}$ with $\left\{I^{(2)},\ J^{(2)}\right\}$ a partition for $J^{(1)}$, *etc.*, until $J^{(L)}$ is empty. This yields

$$\Omega_{i_1\cdots i_K} = U_{I^{(1)}a_1}\cdots U_{I^{(L)}a_L}C_{a_1\cdots a_L}, \tag{S1}$$

where $C_{a_1\cdots a_L} \equiv C^{(L)}_{a_1\cdots a_L}$. Notice that $\{I^{(1)},\ \ldots,\ I^{(L)}\}$ is a partition of the primitive indexes in $\Omega_{i_1\cdots i_K}$. The procedure above is known as the Tucker decomposition.

The Tucker decomposition can further be applied to each $U_{I^{(\ell)}a_\ell}$ with a given $a_\ell$ to get

$$U_{I^{(\ell)}a_\ell} = U'_{I^{(\ell,1)}b_1}\cdots U'_{I^{(\ell,M)}b_M}U^{(1)}_{b_1\cdots b_Ma_\ell}, \tag{S2}$$

with $\{I^{(\ell,1)},\ \ldots,\ I^{(\ell,M)}\}$ to be a partition of $I^{(\ell)}$. Such procedure can be done iteratively until $I^{(\ell,\ m,\ \ldots)}$ only contain one primitive index. This is known as the hierarchical Tucker

decomposition (HTD).[1, 2] Notice that in the expression of such decomposition of a high order tensor, each $U_{Ja}$ satisfies the *semi-unitary* condition

$$U_{Ja}U^{\star}_{Ja'} = \delta_{aa'}, \tag{S3}$$

along the last index, which is inherited from SVD. Because the way of selecting the hierarchical partition in a HTD is not unique, one can easily get various types of HTD for the same high-order tensor.

To precisely represent a HTD of a high-order tensor, we employ the tensor network notation. In the tensor network notation, the set of primitive indexes $\{i_1, \ \ldots, \ i_K\}$ of a $K$-order tensor is bijected to the set of open edges in a tree $G$, and the set of indexes to be summarized in the expression of HTD is bijected to the closed edges in the tree. We define a TTN $(G, \mathcal{V})$ consisting a tree $G = (V, E, R)$ and a valuation function $\mathcal{V}$ for each node $v$ in $G$ with a tensor $\mathcal{V}(v)$ to represent a HTD decomposition of a high order tensor. In the TTN, the valuation $\mathcal{V}(v)$ is called as the *core tensor*. For all node $v \in V$, the degree of $v$ equals to the order of core tensor $\mathcal{V}(v)$. Each edge $a$ attached to the node $v$ corresponds to a index $i_a$ in the expression of HTD. Strictly, the indexes in a core tensor are ordered while the node–edge relation $R(v)$ is disordered, but the correspondence between an index $i_a$ in the tensor network can be bijected to an edge $a$ in tree $G$ by requiring each $R(v)$ is ordered. That is, each $R(v)$ is now extended to a ordered set.

Now we can use the *contraction* of a TTN to represent a HTD of a high-order tensor as $\Omega = \mathsf{Con}(G, \mathcal{V})$. The contraction of a TTN is defined as follows: we first list all core tensor $\mathcal{V}(v)$ for node $v \in V$, each of which is assigned by indexes as $[\mathcal{V}(v)]_{i_{a_1}\cdots i_{a_\mu}}$ if $R(v) = \{a_1, \ \ldots, \ a_\mu\}$. The repeated index label $i_a$ in different $\mathcal{V}(v)$ corresponds to a contracted edge in the graph $G$ and summarized as in the Einsteins summation conversion. The index labels $i_b$ that only appear once become the indexes in the contracted high-order tensor, that is,

$$\Omega_{i_{b_1}\cdots i_{b_K}} = [\mathsf{Con}(G, \mathcal{V})]_{i_{b_1}\cdots i_{b_K}}, \tag{S4}$$

Figure S1 shows three TTN examples that decompose a 4-order tensor $W_{ijkl}$.

If a TTN represents a HTD, from the property of HTD, we can assign one node $r$ as the root of the TTN, such that for any non-root node $u \neq r$, its tensor valuation satisfy the semi-unitary condition Eq. (S3), *i.e.*, $[\mathcal{V}(u)]_{Ji_a}[\mathcal{V}(u)]^{\star}_{Ji'_a} = \delta_{i_a,i'_a}$ for $u \neq r$ where $a$ is the parent edge of $u$.

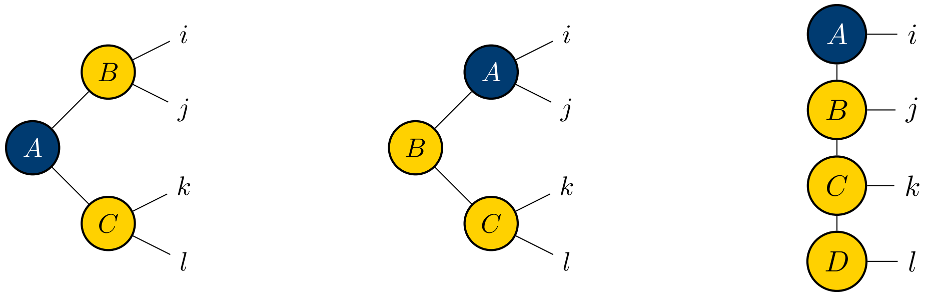


Balanced tensor tree

$W_{ijkl} = A_{mn} B_{ijm} C_{kln}$

Balanced tensor tree

$W_{ijkl} = A_{ijm} B_{nm} C_{kln}$

Tensor train

$W_{ijkl} = A_{ia} B_{bja} C_{ckb} D_{lc}$

FIG. S1. Three possible tree tensor networks for hierarchical Tucker decomposition of a 4-order tensor $W_{ijkl}$. The root node is in blue while non-root vertices are in yellow.

## III. MASTER EQUATION FOR TREE TENSOR NETWORK

For $K$-DoF space $\mathcal{H} = \bigtimes_k \mathcal{H}^{(k)}$ that is constructed from $K$ single DoF space $\mathcal{H}^{(k)}$ with each $\mathcal{H}^{(k)} = \mathbb{C}^{N_k}$. Here $\mathbb{C}$ is set of complex numbers and $N_k$ is the dimension of the $k$-th DoF space. Consider a linear operator $\mathcal{L}$ that maps a $K$-order tensor in $\mathcal{H}$ to another. Suppose that $\mathcal{L}(t) = \sum_m \mathcal{L}_m(t)$ with $\mathcal{L}_m(t) = \bigotimes_k h_m^{(k)}(t)$, where each $h_m^{(k)}(t)$ is a local linear operator that maps a vector in $\mathcal{H}_k$ to another.

For the master equation $\frac{\mathrm{d}}{\mathrm{d}t}\Omega(t) = \mathcal{L}(t)\Omega(t)$ for tensor $\Omega(t)$, as stated in Eq. (17) in the main text, the Dirac–Frenckel time-dependent variational principle is

$$\sum_{i_1 \cdots i_K} [\delta\Omega(t)]^{\star}_{i_1 \cdots i_K} \left[ \left( \mathcal{L}(t) - \frac{\mathrm{d}}{\mathrm{d}t} \right) \Omega(t) \right]_{i_1 \cdots i_K} = 0, \tag{S5}$$

where $\delta\Omega(t)$ is the variation of $\delta\Omega(t)$. Assume that $\Omega(t)$ has a TTN such that $\Omega(t) = \mathsf{Con}(G, \mathcal{V}(t))$ with $\mathcal{V}$ satisfying the semi-unitary condition Eq. (S3) with respect to root $r$ in tree $G$. For non-root node $u$, to preserve the semi-unitary condition Eq. (S3) over the time, we let

$$\frac{\mathrm{d}}{\mathrm{d}t} \sum_I [\mathcal{V}(t,u)]^{\star}_{Ii} [\mathcal{V}(t,u)]_{Ij} = 0, \quad \text{for all } i,\ j. \tag{S6}$$

This can be done by a stronger gauge condition during dynamics[3, 4]

$$\sum_I [\mathcal{V}(t,u)]^{\star}_{Ii} \frac{\mathrm{d}}{\mathrm{d}t} [\mathcal{V}(t,u)]_{Ij} = 0, \quad \text{for all } i,\ j. \tag{S7}$$

This is the generalized requirement as Eq. (18) in the main text.

To give the master equation for each core tensor in TTN, it is convenient to Here $\mathsf{F}^{(a)}_{G,r}(\mathcal{L}_m, \mathcal{V})$ and $\mathsf{D}^{(a)}_{G,r}(\mathcal{L}_m, \mathcal{V})$ depends on $\mathcal{L}_m$ with respect to edge $a$ given valuation $\mathcal{V}$, respectively, for a tree given $G = (V, E, R)$ with root $r$. $\mathsf{F}^{(a)}_{G,r}(\mathcal{L}_m, \mathcal{V})$ and $\mathsf{D}^{(a)}_{G,r}(\mathcal{L}_m, \mathcal{V})$ are the generalization of the $f^{(s)}_m$ and $D^{(s)}_m$ in the main text. Given the tree of the TTN $G$ with root $r$, $\mathsf{F}^{(a)}_{G,r}(\mathcal{L}_m, \mathcal{V})$ and $\mathsf{D}^{(a)}_{G,r}(\mathcal{L}_m, \mathcal{V})$ are defined as follows.

To define $\mathsf{F}^{(a)}_{G,r}(\mathcal{L}_m, \mathcal{V})$ for $\mathcal{L}_m = \bigotimes_k h^{(k)}_m$, the base case is when edge $a$ is open. Suppose $a \in R(u)$ and edge $a$ corresponds to the primitive index $i_a$ in $[h^{(a)}_m]_{i'_a, i_a}$, then

$$[\mathsf{F}^{(a)}_{G,r}(\mathcal{L}_m, \mathcal{V})]_{i_a j_a} \equiv [h^{(a)}_m]_{i_a j_a}. \tag{S8}$$

For an closed edge $a$, then $a$ is the parent edge of some node $u$. Let the parent of $u$ be $v$, and $R(u) = \{a,\ b_1,\ \ldots,\ b_\mu\}$, then

$$[\mathsf{F}^{(a)}_{G,r}(\mathcal{L}_m, \mathcal{V})]_{i_a j_a} \equiv [\mathcal{V}(u)]^\star_{i_{b_1} \cdots i_{b_\mu} i_a} \prod_{\alpha=1}^{\mu} [\mathsf{F}^{(b_\alpha)}_{G,r}(\mathcal{L}_m, \mathcal{V})]_{i_{b_\alpha} j_{b_\alpha}} [\mathcal{V}(u)]_{j_{b_1} \cdots j_{b_\mu} j_a}. \tag{S9}$$

This is the general form of Eq. (21) in the main text.

In turn, to define $\mathsf{D}^{(a)}_{G,r}(\mathcal{L}_m, \mathcal{V})$, the base case is when $a \in R(r)$ is attached to the root $r$, and $R(r) = \{a,\ b_1,\ \ldots,\ b_\mu\}$, then

$$[\mathsf{D}^{(a)}_{G,r}(\mathcal{L}_m, \mathcal{V})]_{i_a j_a} \equiv [V(r)]_{i_a i_{b_1} \cdots i_{b_\mu}} \prod_{\alpha=1}^{\mu} [\mathsf{F}^{(b_\alpha)}_{G,r}(\mathcal{L}_m, \mathcal{V})]_{j_{b_\alpha} i_{b_\alpha}} [V(r)]^\star_{j_a j_{b_1} \cdots j_{b_\mu}}. \tag{S10}$$

For any other edge $a$, suppose $u$ is the node $a \in R(u)$. In this case $u \neq r$. Let $c \in R(u)$ be the parent edge of $u$, and $R(u) = \{a,\ b_1,\ \ldots,\ b_\mu,\ c\}$, then

$$[\mathsf{D}^{(a)}_{G,r}(\mathcal{L}_m, \mathcal{V})]_{i_a j_a} \equiv [\mathcal{V}(u)]_{i_a i_{b_1} \cdots i_{b_\mu} i_c} \left( \prod_{\alpha=1}^{\mu} [\mathsf{F}^{(b_\alpha)}_{G,r}(\mathcal{L}_m, \mathcal{V})]_{j_{b_\alpha} i_{b_\alpha}} \right) [\mathsf{D}^{(c)}_{G,r}(\mathcal{L}_m, \mathcal{V})]_{i_c j_c} [\mathcal{V}(u)]^\star_{j_a j_{b_1} \cdots j_{b_\mu} j_c}, \tag{S11}$$

Equations (S10) and (S11) generalize Eqs. (22)–(24) in the main text. Specially, if $[\mathsf{Con}(G, \mathcal{V})]_{i_1 \cdots i_a \cdots i_K} = \Omega_{i_1 \cdots i_a \cdots i_K}$, then $\mathsf{D}^{(a)}_{G,r}(\hat{1}, \mathcal{V})_{i'_a i''_a} = \Omega_{i_1 \cdots i'_a \cdots \ell_K} \Omega^\star_{i_1 \cdots i''_a \cdots i_K}$. This means that $\mathsf{D}^{(a)}_{G,r}(\hat{1}, \mathcal{V})$ is the reduced density matrix with all DoFs being traced out except for the one corresponds to each $a$. Here $\hat{1}$ is the identity operator. Note that $\mathsf{D}^{(a)}_{G,r}(\hat{1}, \mathcal{V})$ is the generalization of $D^{(s)}$ in the main text.

Now we are ready to give the generalized version of the master equations for each core tensor by substituting the TTN expression $\Omega(t) = \mathsf{Con}(G, \mathcal{V}(t))$ to Eq. (S5), using the fact that the variation of each core tensor is independent and arbitrary. For the root node $r$ with

$R(r) = \{a_1,\ \ldots,\ a_\kappa\}$,

$$\frac{\mathrm{d}}{\mathrm{d}t}[\mathcal{V}(t,r)]_{j_{a_1}\cdots j_{a_\kappa}} = \sum_m \left(\prod_{\alpha=1}^{\kappa}[\mathsf{F}^{(a_\alpha)}_{G,r}(\mathcal{L}_m(t),\mathcal{V}(t))]_{j_{a_\alpha}i_{a_\alpha}}\right)[\mathcal{V}(t,r)]_{j_{a_1}\cdots j_{a_\kappa}}. \tag{S12}$$

This is the generalization of Eq. (19) in the main text.

For the non-root node $u$ with $R(u) = \{a,\ b_1,\ \ldots,\ b_\mu,\}$ where $a$ is the parent edge of $u$,

$$[\mathcal{P}^{(a)}_{G,r}(\mathcal{V}(t))]_{j_a k_a}\frac{\mathrm{d}}{\mathrm{d}t}[\mathcal{V}(t,u)]_{j_a j_{b_1}\cdots j_{b_\mu}} = \sum_m [\mathsf{C}^{(a)}_{G,r}(\mathcal{L}_m(t),\mathcal{V}(t))]_{j_a k_a}\times$$
$$\left(\left(\prod_{\alpha=1}^{\mu}[\mathsf{F}^{(b_\alpha)}_{G,r}(\mathcal{L}_m(t),\mathcal{V}(t))]_{j_{b_\alpha}i_{b_\alpha}}\right)[\mathcal{V}(t,u)]_{j_a i_{b_1}\cdots i_{b_\mu}} - [\mathcal{V}(t,u)]_{i_a j_{b_1}\cdots j_{b_\mu}}[\mathsf{F}^{(a)}_{G,r}(\mathcal{L}_m(t),\mathcal{V}(t))]_{i_a j_a}\right). \tag{S13}$$

Here $\mathsf{C}^{(a)}_{G,r}(\mathcal{L}_m,\mathcal{V})$ is the $C^\star$-adjointness[5] of $\mathcal{L}_m$ given the TTN, which is defined as

$$[\mathsf{C}^{(a)}_{G,r}(\mathcal{L}_m,\mathcal{V})]_{i_a j_a} \equiv [\mathsf{D}^{(a)}_{G,r}(\mathcal{L}_m,\mathcal{V})]_{i_a k_a}[\mathsf{D}^{(a)}_{G,r}(\hat{1},\mathcal{V})^{+}]_{k_a j_a}, \tag{S14}$$

and

$$[\mathcal{P}^{(a)}_{G,r}(\mathcal{V})]_{i_a j_a} \equiv [\mathsf{D}^{(a)}_{G,r}(\hat{1},\mathcal{V})]_{i_a k_a}[\mathsf{D}^{(a)}_{G,r}(\hat{1},\mathcal{V})^{+}]_{k_a j_a} \tag{S15}$$

is a projection matrix to the row space of $\mathsf{D}^{(a)}_{G,r}(\hat{1},\mathcal{V})$. Here $A^+$ denotes the Moore–Penrose inverse of matrix $A$.[6] Eq. (S13) is the general form of Eq. (20) in the main text.

## IV. DIRECT INTEGRATION AND THE REGULARIZATION

The most straightforward propagator is to integrate Eqs. (S12) and (S13) directly. One issue in such propagator is that when calculating $\frac{\mathrm{d}}{\mathrm{d}t}\mathcal{V}(t,u)$ for the non-root node $u$ in Eq. (S13), a possibly singular matrix $\mathcal{P}^{(a)}_{G,r}(\mathcal{V}) \neq \hat{1}$ may occur. This is because $\mathsf{D}^{(a)}_{G,r}(\hat{1},\mathcal{V})$ in Eq. (S14) may be singular, and thus restricts us from getting the exact dynamics of $\mathcal{V}(t,u)$. One way to resolve this problem is to use the regularization process [7–9], such that the dynamical space of $\mathcal{V}(t,u)$ is extended to the null space of $\mathsf{D}^{(a)}_{G,r}(\hat{1},\mathcal{V})$. This can be done from the following process to obtain $\mathsf{C}^{(a)}_{G,r}(\mathcal{L}_m,\mathcal{V}(t))$. This is similar to Eqs. (S10) and (S11).

The base case is when $a \in R(r)$ is attached to the root $r$, and $R(r) = \{a,\ b_1,\ \ldots,\ b_\mu\}$, then firstly we perform the SVD of $\mathcal{V}(r)$ as

$$[\mathcal{V}(r)]_{i_a i_{b_1}\cdots i_{b_\mu}} = W^{(a)}_{j_a i_{b_1}\cdots i_{b_\mu}}\sigma^{(a)}_{j_a}[V^{(a)}]^\star_{i_a j_a}. \tag{S16}$$

We define

$$[\bar{D}^{(a)}]_{i_a j_a} \equiv [V(r)]_{i_a i_{b_1} \cdots i_{b_\mu}} \prod_{\alpha=1}^{\mu} [\mathsf{F}_{G,r}^{(b_\alpha)}(\mathcal{L}_m, \mathcal{V})]_{j_{b_\alpha} i_{b_\alpha}} W^{(a)}_{j_a i_{b_1} \cdots i_{b_\mu}}. \tag{S17}$$

In this case,

$$[\mathsf{C}_{G,r}^{(a)}(\mathcal{L}_m, \mathcal{V})]_{i_a j_a} = [\bar{D}^{(a)}]_{i_a j_a} [\sigma^{(a)}]^{-1}_{j_a} [V^{(a)}]_{j_a i_a}. \tag{S18}$$

For any other edge $a$, suppose it is attached to node $u$ as $a \in R(u)$. In this case $u \neq r$. Let $c \in R(u)$ be the parent edge of $u$, and $R(u) = \{a,\ b_1,\ \ldots,\ b_\mu,\ c\}$, then $\bar{D}^{(c)}$ as well as $W^{(c)}$, $\sigma^{(c)}$ and $V^{(c)}$ are from the SVD of previous steps. Let $A^{(c)}_{i_a i_{b_1} \cdots i_{b_\mu} i_c} \equiv [\mathcal{V}(u)]_{i_a i_{b_1} \cdots i_{b_\mu} j_c} [V^{(c)}]^{\star}_{j_c i_c} \sigma^{(c)}_{i_c}$. The SVD of $A^{(c)}$ gives $W^{(a)}$, $\sigma^{(a)}$, $V^{(a)}$ as

$$A^{(c)}_{i_a i_{b_1} \cdots i_{b_\mu} i_c} = W^{(a)}_{j_a i_{b_1} \cdots i_{b_\mu} i_c} \sigma^{(a)}_{j_a} [V^{(a)}]^{\star}_{i_a j_a}. \tag{S19}$$

We define

$$[\bar{D}^{(a)}]_{i_a j_a} \equiv [\mathcal{V}(u)]_{i_a i_{b_1} \cdots i_{b_\mu} i_c} \left( \prod_{\alpha=1}^{\mu} [\mathsf{F}_{G,r}^{(b_\alpha)}(\mathcal{L}_m, \mathcal{V})]_{j_{b_\alpha} i_{b_\alpha}} \right) [\bar{D}^{(c)}]_{i_c j_c} [W^{(a)}]^{\star}_{j_a j_{b_1} \cdots j_{b_\mu} j_c}. \tag{S20}$$

In this case, Eq. (S18) is also satisfied. Equations (S17) and (S20) generalized Eqs. (30)–(36) in the main text.

The regularization is achieved by the replacing the inverse of singular values in Eq. (S18) by

$$[\mathsf{C}_{G,r}^{(a)}(\mathcal{L}_m, \mathcal{V})]_{i_a j_a} \approx [\bar{D}^{(a)}]_{i_a j_a} [\max(\sigma^{(a)}_{j_a}, \epsilon)]^{-1}_{j_a} [V^{(a)}]_{j_a i_a}, \tag{S21}$$

where $\epsilon$ is a parameter that controls the error introduced by such regularization process. With this regularization, the multiplicative inverse is always achievable. This also gives $\mathcal{P}^{(a)}_{G,r}(\mathcal{V}) \approx \hat{1}$, and is the generalized form of Eq. (42) in the main text.

## V. PROJECTOR-SPLITTING PROPAGATOR

We now introduce the novel projector-splitting propagator which allows us to generate the dynamics of the valuation without using the Eq. (S13) in which the singularity issue may occur. The details of this algorithm, and proof of their validity, are discussed in the studies of tensor train and tensor tree[10–15] in the context of time-evolution of the matrix product state for a wavefunction. Here we briefly outline these algorithms.

As in the main text, the formal solution of the master equation $\frac{\mathrm{d}}{\mathrm{d}t}\Omega(t) = \mathcal{L}(t)\Omega(t)$ is $\Omega(t+\Delta) = e^{\Delta\mathcal{L}(t)}\Omega(t)$ for a small time step $\Delta$. In a Trotterization scheme in PS, $\mathcal{L}(t)$ is split

Algorithm S1. Forward step of PS1.

**for** $i \leftarrow 1,\ 2,\ \ldots,\ L_P - 1$ **do**
  Suppose $P[i]$ is $u$, and $P[i+1]$ is $v$.
  **if** $\mathsf{L}_{G,r}(u) < \mathsf{L}_{G,r}(v)$ **then**
    Call $\texttt{move1}(u, v, 0)$ to update $\mathcal{V}(u)$ and $\mathcal{V}(v)$.
  **else**
    Propagate $\mathcal{V}(u)$ by $\frac{\Delta}{2}$ using Eq. (S12).
    Call $\texttt{move1}(u, v, -\frac{\Delta}{2})$ to update $\mathcal{V}(u)$ and $\mathcal{V}(v)$.
  **end if**
**end for**
Propagate $\mathcal{V}(r)$ by $\frac{\Delta}{2}$ using Eq. (S12).

into $\mathcal{L}(t) = \sum_{i=1}^{I_{\max}} \mathcal{P}_i \mathcal{L}(t)$. The Trotter propagator is $\Omega(t+\Delta) \approx e^{\Delta \mathcal{P}_{I_{\max}} \mathcal{L}(t)} \cdots e^{\Delta \mathcal{P}_1 \mathcal{L}(t)} \Omega(t)$ to first order in $\Delta$, or $\Omega(t+\Delta) \approx e^{\frac{\Delta}{2}\mathcal{P}_1 \mathcal{L}(t)} \cdots e^{\frac{\Delta}{2}\mathcal{P}_{I_{\max}} \mathcal{L}(t)} e^{\frac{\Delta}{2}\mathcal{P}_{I_{\max}} \mathcal{L}(t)} \cdots e^{\frac{\Delta}{2}\mathcal{P}_1 \mathcal{L}(t)} \Omega(t)$ to second order in $\Delta$. We employ the second Trotter where each time step is divided into a forward step in the splitting of $\mathcal{L}$, $e^{\frac{\Delta}{2}\mathcal{P}_{I_{\max}} \mathcal{L}(t)} \cdots e^{\frac{\Delta}{2}\mathcal{P}_1 \mathcal{L}(t)}$, followed by a backward step in such splitting $e^{\frac{\Delta}{2}\mathcal{P}_1 \mathcal{L}(t)} \cdots e^{\frac{\Delta}{2}\mathcal{P}_{I_{\max}} \mathcal{L}(t)}$. We denote each $e^{\tau \mathcal{P}_i \mathcal{L}(t)}$ as a split-step with a time $\tau$.

### A. PS1 algorithm

The key of the algorithm is to find a round-trip path over the whole tensor tree such that each contracted edge in the tree is traveled exactly two times. This can be done by the depth-first-search algorithm[16] from the root $r$. We first travel over the tree: start from the root $r$, go pass every closed edge twice, and return to the origin $r$. The forward path is a sequence $P = (r,\ \ldots,\ u,\ \ldots,\ r)$ with an overall length of $L_P$. We propagate the whole TTN by $\tau/2$ when we travel along the the forward path. After that we use the reversed sequence of the forward path $P$ as the backward path to propagate another $\tau/2$ to finish one step of propagation for the whole TTN. We use $P[i]$ to represent the node at the $i$-th location of the sequence $P$. The forward and backward algorithms are shown in Algorithms S1 and S2.

The algorithms here are similar to the ones in the main text except for the propagation now is based on the generalized form Eq. (S12), and the one-site move function $\texttt{move1}(r, s, \tau)$

Algorithm S2. Backward step of PS1.

```
Propagate 𝒱(r) by Δ/2 using Eq. (S12).
for i ← L_P, L_P − 1, ..., 2 do
    Suppose P[i] is u, and P[i − 1] is v.
    if L_{G,r}(u) < L_{G,r}(v) then
        Propagate 𝒱(u) by Δ/2 using Eq. (S12).
        Call move1(u, v, −Δ/2) to update 𝒱(u) and 𝒱(v).
    else
        Call move1(u, v, 0) to update 𝒱(u) and 𝒱(v).
    end if
end for
```

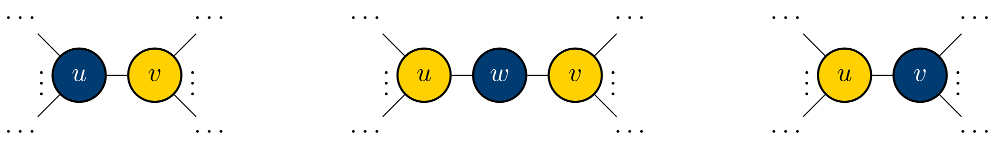


(a) (b) (c)

FIG. S2. Graphic representation of a fragment of TTN during the one site move `move1`$(u, v)$. The root of TTN (a) is $u$ before the move, and after the move the root of TTN (c) is $v$. During the move, a intermediate TTN (b) is constructed. This is done by adding one new temporary root node $w$ to the graph and inserting in the contracted edge between $u$ and $v$.

is now extended to arbitrary tree as showed in Algorithm S3. Notice that during Algorithm S3, the following master equation is used for propagating the matrix $M$

$$\frac{\mathrm{d}}{\mathrm{d}t} M_{i'_a j'_a} = \sum_m [\mathsf{F}^{(a)}_{G,v}(\mathcal{L}_m, \mathcal{V})]_{i'_a i_a} [\mathsf{F}^{(a)}_{G,u}(\mathcal{L}_m, \mathcal{V})]_{j'_a j_a} M_{i_a j_a}. \tag{S22}$$

Notice that during the `move1`, it can be understood as an intermediate TTN $(G', \mathcal{V}')$ with the root at a new node $w$ inserted between $u$ and $v$ is constructed. In this intermediate TTN, the valuation $\mathcal{V}'(w) = M$ while $\mathcal{V}'(u) = U$. The valuation of all other nodes $s \neq u$ that occurs in the original TTN $G$ remains the same $\mathcal{V}'(s) = \mathcal{V}(s)$. The graphic representation is showed in Fig. S2.

Algorithm S3. One-site move function $\texttt{move1}(r, s, \tau)$.

// *Assuming $u$ is the root of TTN $(G, \mathcal{V})$, and $v$ is in the neighborhood of $u$.*

// *Suppose $R(u) = \{a,\ b_1,\ \ldots,\ b_\mu\}$ and $R(v) = \{a,\ c_1,\ \ldots,\ c_\nu\}$.*

Let $A_{Ij_a} \leftarrow [\mathcal{V}(u)]_{j_a i_{b_1} \cdots i_{b_\mu}}$ with $I = \{i_{b_1},\ \ldots,\ i_{b_\mu}\}$.

Calculate the SVD $A_{Ij_a} = U_{Ik_a} \sigma_{k_a} V^\star_{j_a k_a}$.

Let $U'_{k_a i_{b_1} \cdots i_{b_\mu}} \leftarrow U_{Ik_a}$.

Update $\mathcal{V}(u) \leftarrow U'$.

Let $M_{j_a k_a} \leftarrow V^\star_{j_a k_a} \sigma_{k_a}$.

Propagate $M$ by $\tau$ using Eq. (S22).

Let $V'_{i_{b_1} \cdots i_{b_\mu} k_a} \leftarrow M_{j_a k_a} [\mathcal{V}(v)]_{j_a i_{b_1} \cdots i_{b_\mu}}$.

Update $\mathcal{V}(v) \leftarrow V'$.

Algorithm S4. Forward step of PS2.

**for** $i \leftarrow 1,\ 2,\ \ldots,\ L_p - 1$ **do**

  Suppose $P[i]$ is $u$, and $P[i+1]$ is $s$.

  **if** $\mathsf{L}_{G,r}(u) < \mathsf{L}_{G,r}(v)$ **then**

    Call $\texttt{move1}(u, v, 0)$ to update $\mathcal{V}(u)$ and $\mathcal{V}(v)$.

  **else**

    Call $\texttt{move2}(u, v, \frac{\Delta}{2})$ to update $\mathcal{V}(u)$ and $\mathcal{V}(v)$.

    Propagate $\mathcal{V}(v)$ by $-\frac{\Delta}{2}$ using Eq. (S12).

  **end if**

**end for**

Propagate $\mathcal{V}(r)$ by $\frac{\Delta}{2}$ use Eq. (S12).

### B. PS2 algorithm

In the two-site PS algorithm (PS2), the forward steps and backward steps are similar to those in PS1, but PS2 implements a two-site move of the root tensor in the split steps in addition to the one-site move. The iterative PS2 algorithm for the forward step in the splitting of $\mathcal{L}$ is showed in Algorithm S4, and the backward one in Algorithm S5.

As in the PS1, the PS2 algorithms here are also similar to the ones in the main text except

Algorithm S5. Backward step of PS2.

```
Propagate V(r) by Δ/2 use Eq. (S12).
for i ← L_P, L_P − 1, ..., 2 do
    Suppose P[i] is u, and P[i − 1] is v.
    if L_{G,r}(u) < L_{G,r}(v) then
        Propagate V(u) by −Δ/2 using Eq. (S12).
        Call move2(u, v, Δ/2) to update V(u) and V(v).
    else
        Call move1(u, v, 0) to update V(u) and V(v).
    end if
end for
```

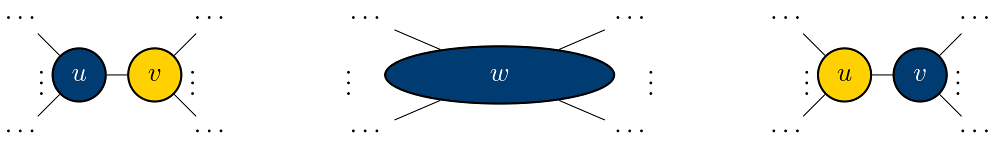


(a) (b) (c)

FIG. S3. Graphic representation of a fragment of TTN during the two-site move move2$(u, v)$. Before the move, the TTN (a) has a root at $u$ and after the move the root of TTN (c) is at $v$. During the move, a intermediate TTN (b) is constructed. This is done by merging the nodes $u$ and $v$ as a new temporary root node $w$.

that the propagation now is based on the generalized form Eq. (S12), and the two-site move function move2$(r, s, \tau)$ is now also extended to arbitrary tree as showed in Algorithm S6. During Algorithm S3, the following master equation is used for propagating the tensor $M$

$$\frac{\mathrm{d}}{\mathrm{d}t} M_{i'_{b_1}\cdots i'_{b_\mu} j'_{c_1}\cdots j'_{c_\nu}} = \sum_m \prod_{\alpha=1}^{\mu} [\mathsf{F}_{G,v}^{(b_\alpha)}(\mathcal{L}_m, \mathcal{V})]_{i'_{b_\alpha} i_{b_\alpha}} \prod_{\beta=1}^{\nu} [\mathsf{F}_{G,u}^{(c_\beta)}(\mathcal{L}_m, \mathcal{V})]_{j'_{c_\beta} j_{c_\beta}} M_{i_{b_1}\cdots i_{b_\mu} j_{c_1}\cdots j_{c_\nu}}. \quad \text{(S23)}$$

Notice that during the move2, it can be understood as an intermediate TTN $(G', \mathcal{V}')$ with the root at a new node $w$ merged from node $u$ and $v$ is constructed. This intermediate TTN, the tensor $\mathcal{V}'(w) = M$. The valuation of all other nodes $s \neq u$ that occurs in the original TTN $G$ remains the same $\mathcal{V}'(s) = \mathcal{V}(s)$. The graphic representation is showed in Fig. S3.

For the PS2 propagation scheme, the overall computational complexity much higher as it propagates over higher order tensors that are from contracting two connected tensors. That

Algorithm S6. Two-site move function $\texttt{move2}(r, s, \tau)$.

// *Assuming $u$ is the root of TTN $(G, \mathcal{V})$, and $v$ is in the neighborhood of $u$.*

// *Suppose $R(u) = \{a,\ b_1,\ \ldots,\ b_\mu\}$ and $R(v) = \{a,\ c_1,\ \ldots,\ c_\nu\}$.*

1. Let $M_{i_{b_1}\cdots i_{b_\mu} j_{c_1}\cdots j_{c_\nu}} \leftarrow [\mathcal{V}(u)]_{k_a i_{b_1}\cdots i_{b_\mu}} [\mathcal{V}(v)]_{k_a j_{c_1}\cdots j_{c_\nu}}$.
2. Propagate $M$ by $\tau$ using Eq. (S23).
3. Let $A_{IJ} \leftarrow M_{i_{b_1}\cdots i_{b_\mu} j_{c_1}\cdots j_{c_\nu}}$ with $I = \{i_{b_1},\ \ldots,\ i_{b_\mu}\}$ and $J = \{j_{c_1},\ \ldots,\ j_{c_\nu}\}$.
4. Calculate the SVD $A_{IJ} = U_{Ik_a} \sigma_{k_a} V^\star_{Jk_a}$.
5. Let $U'_{k_a i_{b_1}\cdots i_{b_\mu}} \leftarrow U_{Ik_a}$.
6. Let $V'_{\ell_a j_{c_1}\cdots i_{c_\nu}} \leftarrow \sigma_{\ell_a} V^\star_{J\ell_a}$.
7. Update $\mathcal{V}(u) \leftarrow U'$ and $\mathcal{V}(v) \leftarrow V'$

is, $(d_1 + d_2 - 2)$-order tensors are propagated during $\texttt{move2}(u, v, \tau)$ if the tensor $\mathcal{V}(u)$ and $\mathcal{V}(v)$ are of order $d_1$ and $d_2$, respectively.


[1] L. Grasedyck, SIAM Journal on Matrix Analysis and Applications **31**, 2029 (2010).

[2] L. Grasedyck and W. Hackbusch, Computational Methods in Applied Mathematics **11**, 291 (2011).

[3] H.-D. Meyer, U. Manthe, and L. S. Cederbaum, Chem. Phys. Lett. **165**, 73 (1990).

[4] H. Wang and M. Thoss, J. Chem. Phys. **119**, 1289 (2003).

[5] D. Viennot, Journal of Geometry and Physics **133**, 42 (2018).

[6] R. Penrose, Mathematical Proceedings of the Cambridge Philosophical Society **51**, 406 (1955).

[7] H.-D. Meyer and H. Wang, J. Chem. Phys. **148**, 124105 (2018).

[8] H. Wang and H.-D. Meyer, J. Chem. Phys. **149**, 44119 (2018).

[9] H. Wang and H.-D. Meyer, The Journal of Physical Chemistry A **125**, 3077 (2021).

[10] J. Haegeman, C. Lubich, I. Oseledets, B. Vandereycken, and F. Verstraete, Phys. Rev. B **94**, 165116 (2016).

[11] B. Kloss, I. Burghardt, and C. Lubich, J. Chem. Phys. **146**, 174107 (2017).

[12] C. Lubich, I. Oseledets, and B. Vandereycken, SIAM J. Numer. Anal. **53**, 917 (2015).

[13] C. Lubich, B. Vandereycken, and H. Walach, SIAM J. Numer. Anal. **56**, 1273 (2018).

[14] L. P. Lindoy, B. Kloss, and D. R. Reichman, The Journal of Chemical Physics **155**, 10.1063/5.0070042 (2021).

[15] L. P. Lindoy, B. Kloss, and D. R. Reichman, The Journal of Chemical Physics **155**, 10.1063/5.0070043 (2021).

[16] R. Tarjan, SIAM Journal on Computing **1**, 146 (1972).
